# Supplementary material for: Constraints on the latitudinal profile of Jupiter's deep jets
Source: arXiv:2102.10595 source file (2021-02-21)
Supplement: Supplementary file 1 [file Galanti_2021_SI_GRL_submitted.pdf]

# Supporting Information for: “Constraints on the latitudinal profile of Jupiter’s deep jets”

Eli Galanti<sup>1</sup>, Yohai Kaspi<sup>1</sup>, Keren Duer<sup>1</sup>, Leigh Fletcher<sup>2</sup>, Andrew Ingersoll<sup>3</sup>,  
Cheng Li<sup>4</sup>, Glenn S. Orton<sup>5</sup>, Tristan Guillot<sup>6</sup>, Steven .M. Levin<sup>5</sup> and Scott J. Bolton<sup>7</sup>

(draft)

February 9, 2021

<sup>1</sup>*Department of Earth and Planetary Sciences, Weizmann Institute of Science, Rehovot, Israel.*

<sup>2</sup>*School of Physics and Astronomy, University of Leicester, Leicester, UK*

<sup>3</sup>*California Institute of Technology, Pasadena, CA, USA*

<sup>4</sup>*Department of Climate and Space Sciences and Engineering, University of Michigan, Ann Arbor, MI, USA*

<sup>5</sup>*Jet Propulsion Laboratory, California Institute of Technology, Pasadena, USA*

<sup>6</sup>*Observatoire de la Cote d’Azur, Nice, France*

<sup>7</sup>*Southwest Research Institute, San Antonio, Texas, TX, USA*

## S1 Model setup

### S1.1 The modified cloud-level wind

Similar to the approach taken in *Kaspi et al.* [2020] and *Galanti and Kaspi* [2021], we look for a slightly modified cloud-level wind that will allow an exact fit to the odd gravity harmonics  $J_3$ ,  $J_5$ ,  $J_7$ , and  $J_9$ . This is done in order to single out the dependence of the wind-induced gravity harmonics on the latitudinal variability of the wind that is examined in the study. This is done by decomposing the observed cloud-level wind into Legendre polynomials

$$U^{\text{obs}}(\theta) = \sum_{i=0}^N A_i^{\text{obs}} P_i(\sin \theta), \quad (1)$$

where  $A_i^{\text{obs}}$  are the coefficients determining the latitudinal shape of the observed wind,  $P_i$  are the Legendre polynomials, and  $N = 99$  is the number of polynomials to be used. The  $A_i^{\text{obs}}$  are calculated from the observed cloud-level wind of *Tollefson et al.* [2017]. Defining a modified cloud-level wind

$$U^{\text{sol}}(\theta) = \sum_{i=0}^N A_i^{\text{sol}} P_i(\sin \theta), \quad (2)$$

where  $A_i^{\text{sol}}$  are the modified coefficients, we allow these coefficients to vary during the optimization process (see below, section S1.4). Note that we construct the wind using a very large number of polynomials. This is done in order to allow the wind solution to follow closely the observed wind. The optimization procedure described below ensures that the this large number of coefficients is well constrained.

Since the observed wind [*Tollefson et al.*, 2017] already allows a very good match to the observed odd gravity harmonics [*Kaspi et al.*, 2018, see also Fig. 4 in the main text], only slight modifications are needed to enable an exact fit (Fig. S1a). The deviation of the optimized wind is well within the observed uncertainty of around  $15 \text{ m s}^{-1}$  [*Tollefson et al.*, 2017]. In the case where the inner part of the decay function is fixed to allow compatibility to magnetic secular variations (Fig 5g in the main text), the optimized cloud-level wind, while a little farther away, is again within the uncertainty of the observed wind (Fig. S1b).

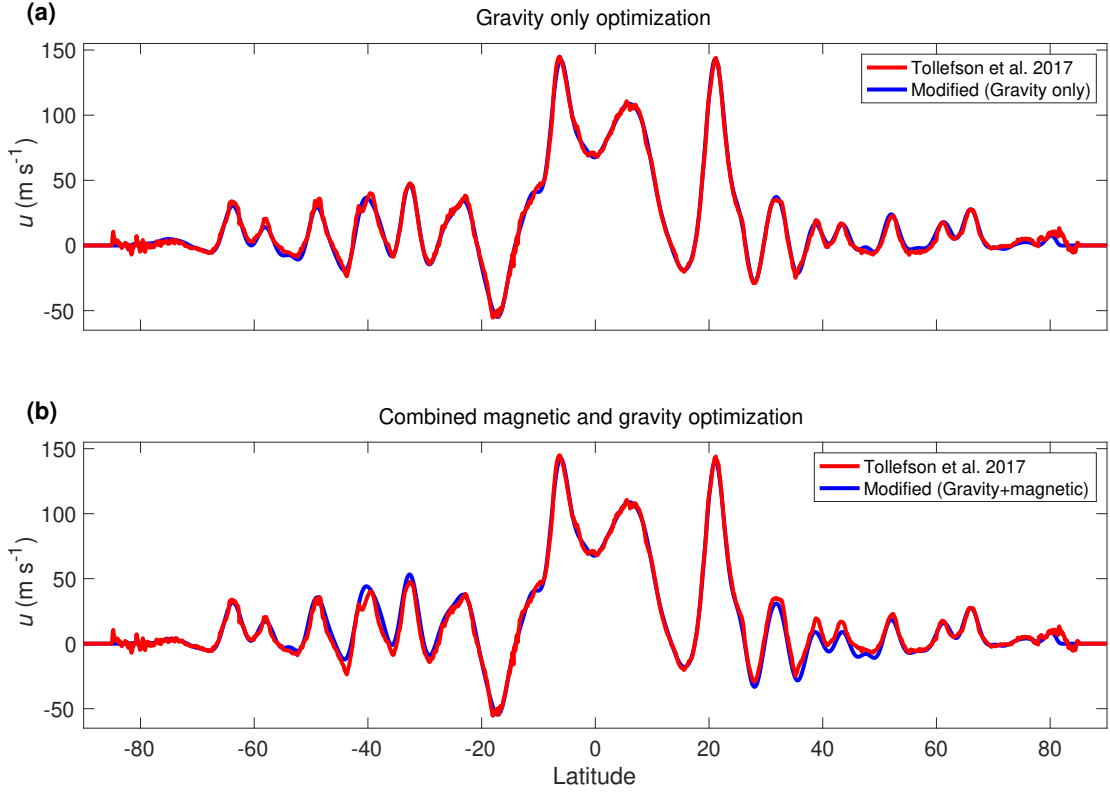

Figure S1: The cloud-level winds used in the study (blue), shown together with the observed wind [Tollefson *et al.*, 2017, red]. (a) The wind optimized to allow an exact fit to the odd gravity harmonics only. (b) The wind optimized to allow an exact fit the odd gravity harmonics when the decay function in the semiconducting region is fixed according to magnetic secular variations. See Galanti and Kaspi [2021] for a detailed derivation and discussion.

## S1.2 The flow field below the cloud level

We start by extending the cloud-level wind (Fig. S1) into the interior, keeping constant values along lines parallel to the spin axis. Then, we allow the flow to decay in the radial direction. The resulting flow field can be defined as

$$u(r, \theta) = u_{\text{cyl}}(s)Q(r), \quad (3)$$

where  $u_{\text{cyl}}(s)$  is the cloud-level zonal wind projected downward parallel to the spin axis and  $s = r \cos(\theta)$  is the distance from the axis of rotation. The radial decay function  $Q(r)$  is defined as

$$Q(r) = (1 - \alpha) \exp\left(\frac{r - R_e}{H}\right) + \alpha \left[ \frac{\tanh\left(-\frac{R_e - H - r}{\Delta H}\right) + 1}{\tanh\left(\frac{H}{\Delta H}\right) + 1} \right], \quad (4)$$

where  $H$  is the scale height,  $\alpha$  is the contribution ratio between an exponential and a normalized hyperbolic tangent function, and  $\Delta H$  is the width of the hyperbolic tangent. These are the parameters that are searched for during the optimization process.

In the case where MHD considerations are taken into account (section 5 in main text), the decay function  $Q(r)$  is defined as

$$Q(r) = \tanh\left(\frac{r - R_T}{\delta H_T}\right) \frac{1 - f_M}{\tanh\left(\frac{R - R_T}{\delta H_T}\right)} + f_M, \quad R_T < r < R, \quad (5)$$

$$Q(r) = f_M \exp\left(\frac{r - R_T}{H_M}\right), \quad r \leq R_T, \quad (6)$$

where  $\delta H_T$  is the width of the hyperbolic tangent function,  $f_M$  is the ratio between the flow strength at the transition depth and the flow at the cloud-level and  $H_M$  is the decay scale-height in the inner layer [Cao and Stevenson, 2017]. This functional form of the flow's radial decay allows two distinctly different behaviors in the regions above and

below the transition depth  $R_T$ . In the outer region the decay function represents a non-magnetic dynamical effect, with the baroclinic shear being in thermal wind balance [Kaspi et al., 2009], and the free parameter  $\delta H_M$  allowing a range of decaying profiles, from a gradual decay to a case where the cloud-level winds keep their value almost constant until reaching the transition depth. In the inner region, the exponential decay function is assumed to be a result of the increased electrical conductivity  $\sigma$ .

The above assumptions are modified in two cases examined in the study. In the first case, the cloud-level wind is projected inward in the radial direction, defined as

$$u(r, \theta) = U^{\text{obs}}(\theta)Q(r), \quad (7)$$

where  $U^{\text{obs}}(\theta)$  is the observed cloud-level wind. In the second case, the wind is projected inward parallel to the spin axis, but is decayed also in the same direction, so that

$$Q(\theta, r) = (1 - \alpha) \exp\left(\frac{-z(\theta, r)}{H}\right) + \alpha \left[ \frac{\tanh\left(-\frac{z(\theta, r) - H}{\Delta H}\right) + 1}{\tanh\left(\frac{H}{\Delta H}\right) + 1} \right], \quad (8)$$

where

$$z(r, \theta) = (R_e - r) \sin \theta. \quad (9)$$

In both cases, the same three parameters,  $H$ ,  $\alpha$  and  $\Delta H$ , are optimized to give the best fit to the gravity harmonics.

### S1.3 The wind-induced gravity

In large-scale flow on fast-rotating planets, such as Jupiter, there exists a balance between the anomalous density field  $\rho'$  and the flow field  $u$ . Here we give a short version of the derivation of this balance (for the full derivation refer to Kaspi et al., 2018). Consider the full momentum balance on a rotating planet

$$\frac{\partial \mathbf{u}}{\partial t} + (\mathbf{u} \cdot \nabla) \mathbf{u} + 2\mathbf{\Omega} \times \mathbf{u} + \mathbf{\Omega} \times \mathbf{\Omega} \times \mathbf{r} = -\frac{1}{\rho} \nabla p + \nabla \Phi, \quad (10)$$

where  $\mathbf{u}$  is the 3D flow vector,  $\mathbf{\Omega}$  is the planetary rotation rate,  $\rho$  is density,  $p$  is pressure and  $\Phi$  is the body force potential set by gravity so that  $\nabla \Phi = -\mathbf{g}$  [Pedlosky, 1987]. It can be shown that under the assumption of a small Rossby number (large scale motions on a fast rotating planet) and a steady state, the equations governing the flow can be written as that

$$2\mathbf{\Omega} \times (\rho \mathbf{u}) = -\nabla p - \rho \mathbf{g} - \rho \mathbf{\Omega} \times \mathbf{\Omega} \times \mathbf{r}. \quad (11)$$

Separating the solutions to a rigid body solution  $\rho_s(r, \theta)$ ,  $p_s(r, \theta)$ , and  $\mathbf{g}_s(r, \theta)$  in which  $\mathbf{u} = 0$ , and a deviation due to the dynamics  $\rho'(r, \theta)$ ,  $p'(r, \theta)$ , and  $\mathbf{g}'(r, \theta)$ , the dynamical balance becomes

$$2\mathbf{\Omega} \times (\rho_s \mathbf{u}) = -\nabla p' - \rho_s \mathbf{g}' - \rho' \mathbf{g}_s - \rho' \mathbf{\Omega} \times \mathbf{\Omega} \times \mathbf{r}. \quad (12)$$

Next, neglecting all terms including  $g'$  (scale analysis of the terms), and taking the curl we get

$$2\mathbf{\Omega} \cdot \nabla (\rho_s \mathbf{u}) = \nabla \rho' \times \mathbf{g}. \quad (13)$$

Lastly, taking the flow to be zonally symmetric  $\mathbf{u} = u(r, \theta) \hat{\phi}$ , the balance becomes

$$2\Omega r \frac{\partial}{\partial z} (\rho_s u) = g_s \frac{\partial \rho'}{\partial \theta}, \quad (14)$$

where  $\theta$  and  $z$  are the latitudinal and axis of rotation directions, respectively. If the flow field  $u$  is known then this equation can be solved for  $\rho'$  up to an integration constant  $\bar{\rho}(r)$  that does not affect the gravity harmonics (again, see Kaspi et al., 2018 for a detailed derivation). This balance was used extensively to study the wind structure on Jupiter [e.g., Kaspi, 2013; Liu et al., 2013; Zhang et al., 2015; Galanti and Kaspi, 2016; Kaspi et al., 2016; Galanti et al., 2017; Kaspi et al., 2018], as well as for the prediction of the wind-induced gravity field to be expected on Jupiter [Kaspi, 2013; Galanti et al., 2017]. The wind-induced gravity harmonics are calculated as the volume integral of  $\rho'$  projected onto Legendre polynomials

$$\Delta J_n = \frac{2\pi}{MR_e^n} \int_0^{R_e} r^{n+2} dr \int_{\theta=-\pi/2}^{\pi/2} P_n(\sin \theta) \rho'(r, \theta) \cos \theta d\theta. \quad (15)$$

## 74 S1.4 The optimization process

75 First, we discuss the optimization procedure used to calculate the optimal cloud-level wind (section S1.1). For more  
 76 details on the optimization methodology refer to [Galanti and Kaspi, 2016, 2021]. The parameters to be optimized,  
 77 i.e., those defining the depth of the wind and the cloud-level wind latitudinal profile, are defined as a control vector

$$\mathbf{X}_C = \{\mathbf{X}_H, \mathbf{X}_U\} = \{[H_0/h_{\text{nor}}, \Delta H/h_{\text{nor}}, \alpha/\alpha_{\text{nor}}], [A_1^{\text{sol}}, \dots, A_N^{\text{sol}}]/u_{\text{nor}}\}, \quad (16)$$

78 where  $H_0$ ,  $\Delta H$  and  $\alpha$  are the parameters defining the radial decay of the wind,  $A_i^{\text{sol}}$  are the parameters defining  
 79 the cloud-level wind, and  $h_{\text{nor}} = 10^7$ ,  $\alpha_{\text{nor}} = 1$ , and  $u_{\text{nor}}10^3$  are the normalization factors for the depth of the  
 80 wind, the mixing coefficient, and the wind coefficients, respectively. The normalization factors are chosen so that  
 81  $-1 < H_0/h_{\text{nor}}, \Delta H/h_{\text{nor}}, \alpha/\alpha_{\text{nor}}, A_i^{\text{sol}}/u_{\text{nor}} < 1$ .

82 The goal is to minimize the difference between the model solution for the gravity field and that measured by Juno,  
 83 given the uncertainties of the measurements, and the need to keep the optimized control parameters regularized to  
 84 physical values. The cost function to be minimized is therefore

$$L = (\mathbf{J}^{\text{m}} - \mathbf{J}^{\text{o}})\mathbf{W}(\mathbf{J}^{\text{m}} - \mathbf{J}^{\text{o}})^{\text{T}} + \epsilon_H \mathbf{X}_H \mathbf{X}_H^{\text{T}} + \epsilon_U (\mathbf{X}_U - \mathbf{X}_0)(\mathbf{X}_U - \mathbf{X}_0)^{\text{T}}, \quad (17)$$

85 where  $\mathbf{J}^{\text{m}} = [J_3^{\text{m}}, J_5^{\text{m}}, J_7^{\text{m}}, J_9^{\text{m}}]$  and  $\mathbf{J}^{\text{o}} = [J_3^{\text{o}}, J_5^{\text{o}}, J_7^{\text{o}}, J_9^{\text{o}}]$  are the calculated and measured gravity harmonics [Iess  
 86 *et al.*, 2018], respectively,  $\mathbf{X}_0 = [A_1^{\text{obs}}, \dots, A_{99}^{\text{obs}}]/u_{\text{nor}}$  are the observed wind profile parameters,  $\epsilon_H = 2 \cdot 10^9$  is the  
 87 weight given to the regularization of the depth parameters, and  $\epsilon_U = 5 \cdot 10^8$  is the weight given to the regularization  
 88 of the wind solution to the observed one. The cost function is composed of three terms, the first is the difference  
 89 between the measured and calculated gravity harmonics, the second assures that the depth of the wind solution  
 90 does not depend on the initial guess, and the third assures that the wind solution does not vary too far from the  
 91 observed one. Given the value of  $\epsilon_U$  and the large number of coefficients defining the wind latitudinal profile, the  
 92 regularization of the wind is very strong, thus ensuring that deviations from the observed cloud-level wind are  
 93 allowed only if they result in a significantly lower value of the cost function. Given an initial guess for  $\overrightarrow{\mathbf{X}_C}$ , a  
 94 minimal value of  $L$  is searched for using the Matlab function 'fmincon' and taking advantage of the cost-function  
 95 gradient that is calculated with the adjoint of the dynamical model [Galanti and Kaspi, 2016].

96 Then, in the experiments conducted in section 3 to 5 of the main text, the cloud-level wind is fixed, so that the  
 97 cost function is set to

$$L = (\mathbf{J}^{\text{m}} - \mathbf{J}^{\text{o}})\mathbf{W}(\mathbf{J}^{\text{m}} - \mathbf{J}^{\text{o}})^{\text{T}} + \epsilon_H \mathbf{X}_H \mathbf{X}_H^{\text{T}}, \quad (18)$$

98 where  $\mathbf{J}^{\text{m}} = [J_3^{\text{m}}, J_5^{\text{m}}, \Delta J_6^{\text{m}}, J_7^{\text{m}}, \Delta J_8^{\text{m}}, J_9^{\text{m}}, \Delta J_{10}^{\text{m}}]$  and  $\mathbf{J}^{\text{o}} = [J_3^{\text{o}}, J_5^{\text{o}}, \Delta J_6^{\text{o}}, J_7^{\text{o}}, \Delta J_8^{\text{o}}, J_9^{\text{o}}, \Delta J_{10}^{\text{o}}]$ . The goal here is to  
 99 fit not only the odd harmonics, but all the residual even harmonics (see main text). Note that the cost function  
 100 presented in the results (e.g., Fig. 3a in main text) includes only the first term of Eq. 18 that gives the direct  
 101 measure for the model solution.

## S2 Solutions with variants of the flow structures

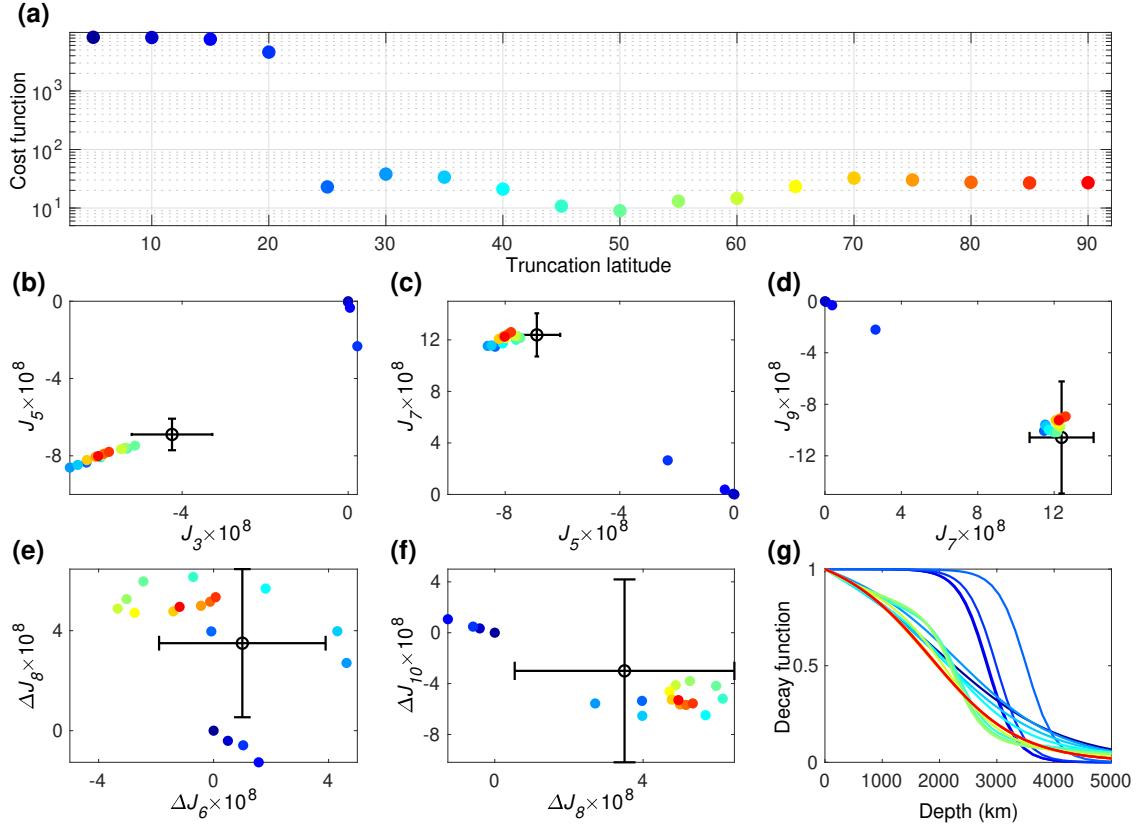

Figure S2: **Similar to Fig. 3 in the main text, but for solutions with the *Tollefson et al.* [2017] cloud-level winds.** Latitude-dependent solutions, as function of the cutoff latitude. (a) The overall fit of the model solution to the measurements (cost function). Each case is assigned with a different color, used in the following panels. (b-f) the solutions for the different gravity harmonics (colors), and the measurement (black). (g) the decay function associated with each solution.

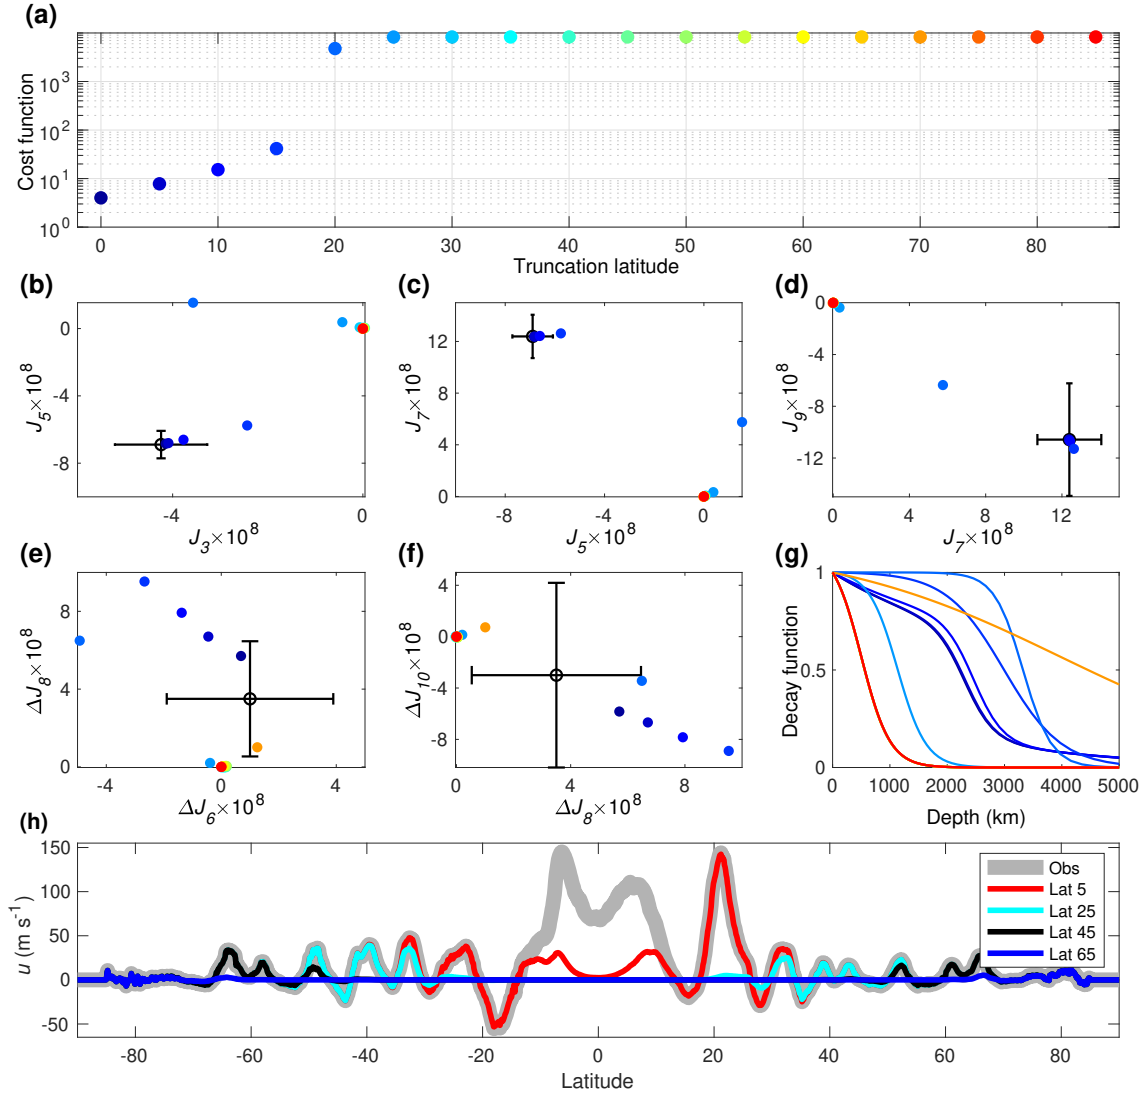

Figure S3: **Solutions with the cloud-level wind truncated inside a latitudinal region.** We examine 18 cases in which the cloud-level wind is truncated equatorward of a certain latitude, for example, set to zero inside the  $25^\circ\text{S}$ - $25^\circ\text{N}$  region (see panel h). (a) The overall fit of the model solution to the measurements (cost function). Each case is assigned with a different color, used in the following panels. (b-f) the solutions for the different gravity harmonics (colors), and the measurement (black). (g) the decay function associated with each solution. The analysis shows that a wind truncated equatorward of a latitude larger than  $20^\circ\text{S}$ - $20^\circ\text{N}$  does not allow a plausible solution to be reached. (h) Examples of wind truncated equatorward of latitude  $5^\circ$ ,  $25^\circ$ ,  $45^\circ$ , and  $65^\circ$ .

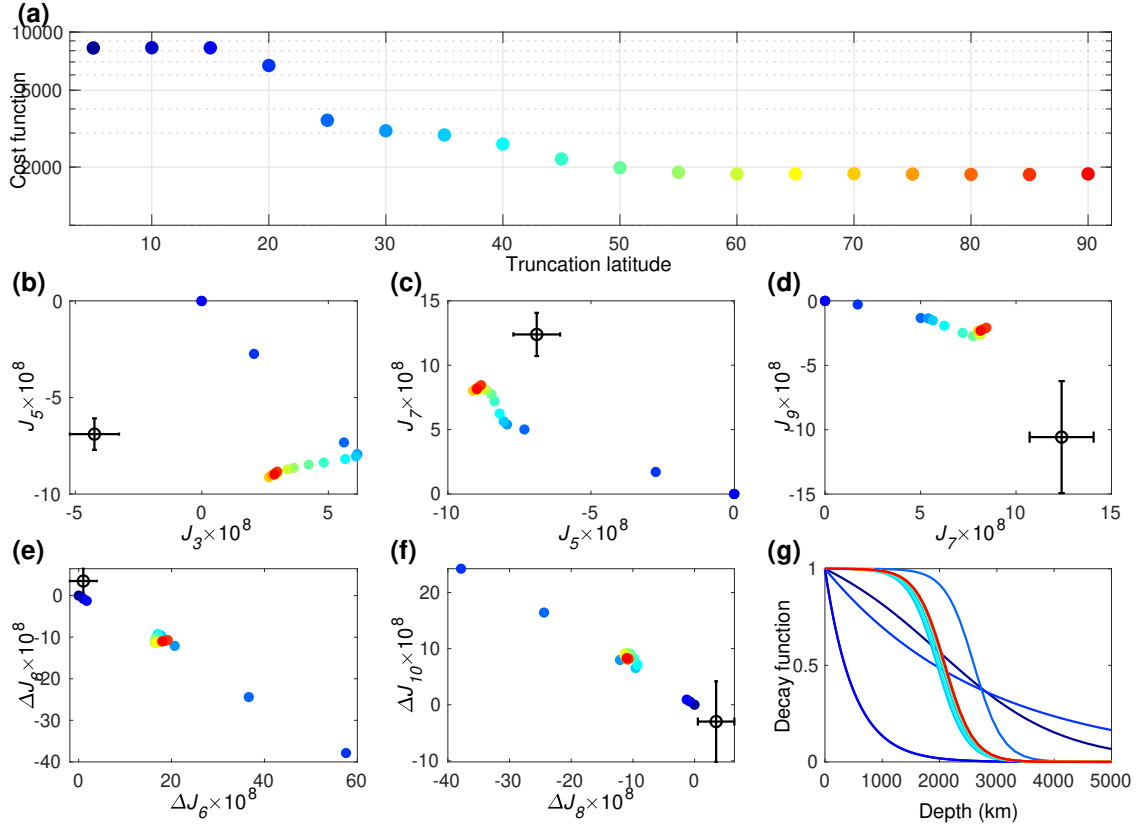

Figure S4: **Similar to Fig. 3 in the main text, but for solutions with radial projection of the observed cloud-level winds.** Latitude-dependent solutions, as function of the cutoff latitude. (a) The overall fit of the model solution to the measurements (cost function). Each case is assigned with a different color, used in the following panels. (b-f) the solutions for the different gravity harmonics (colors), and the measurement (black). (g) the decay function associated with each solution.

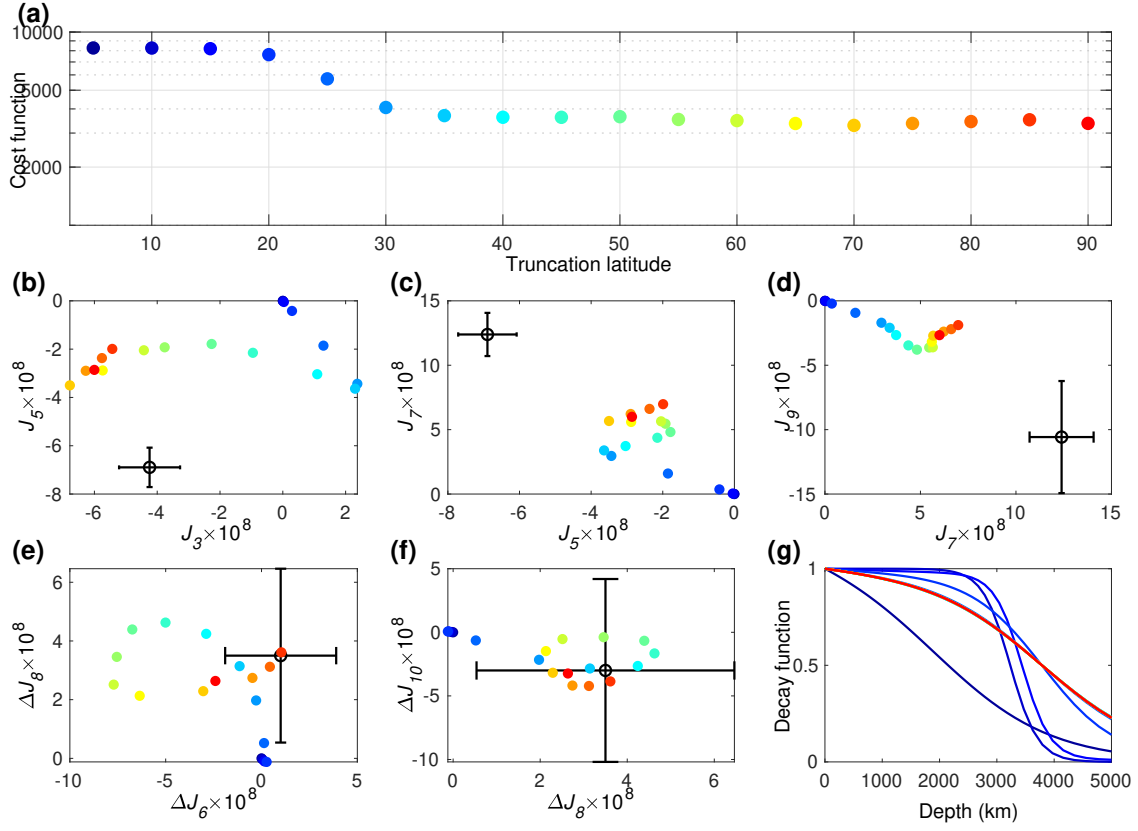

Figure S5: **Similar to Fig. 3 in the main text, but for solutions with wind decay in the Z direction.** Latitude-dependent solutions, as function of the cutoff latitude. (a) The overall fit of the model solution to the measurements (cost function). Each case is assigned with a different color, used in the following panels. (b-f) the solutions for the different gravity harmonics (colors), and the measurement (black). (g) the decay function associated with each solution.

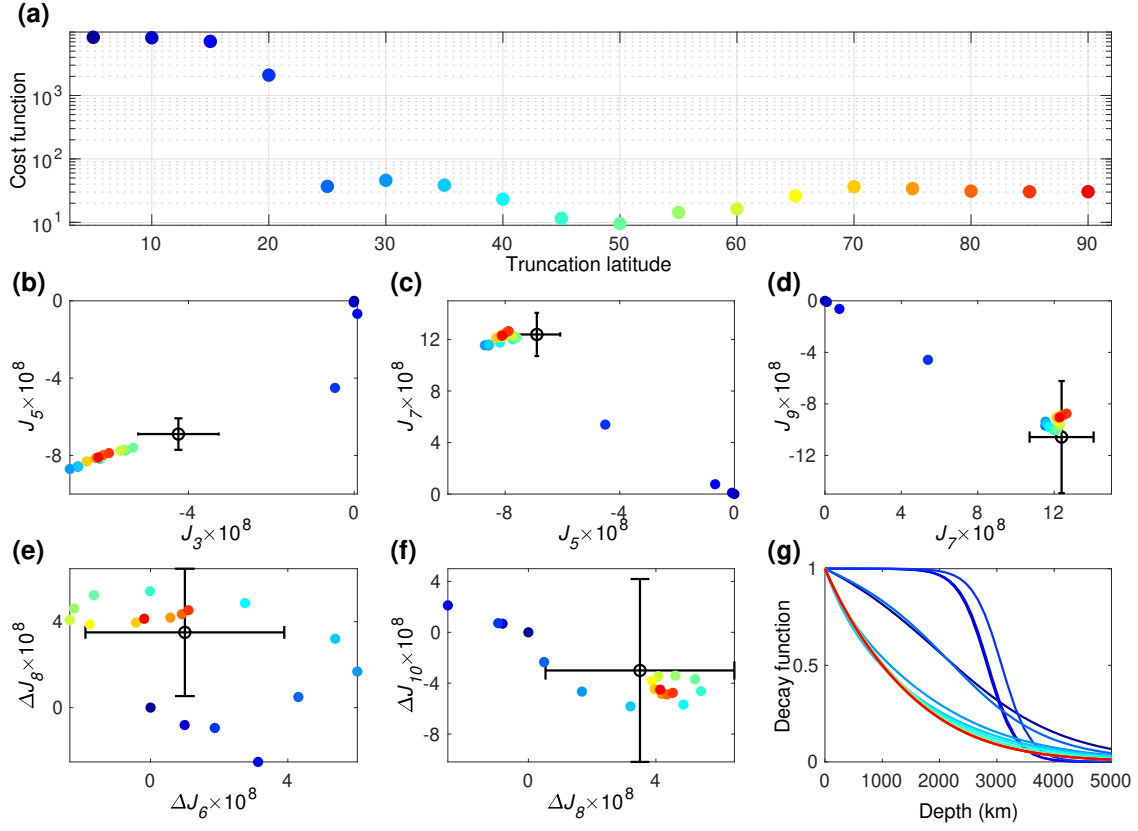

Figure S6: **Similar to Fig. 3 in the main text, but for solutions with doubled cloud-level winds.** Latitude-dependent solutions, as function of the cutoff latitude. (a) The overall fit of the model solution to the measurements (cost function). Each case is assigned with a different color, used in the following panels. (b-f) the solutions for the different gravity harmonics (colors), and the measurement (black). (g) the decay function associated with each solution.

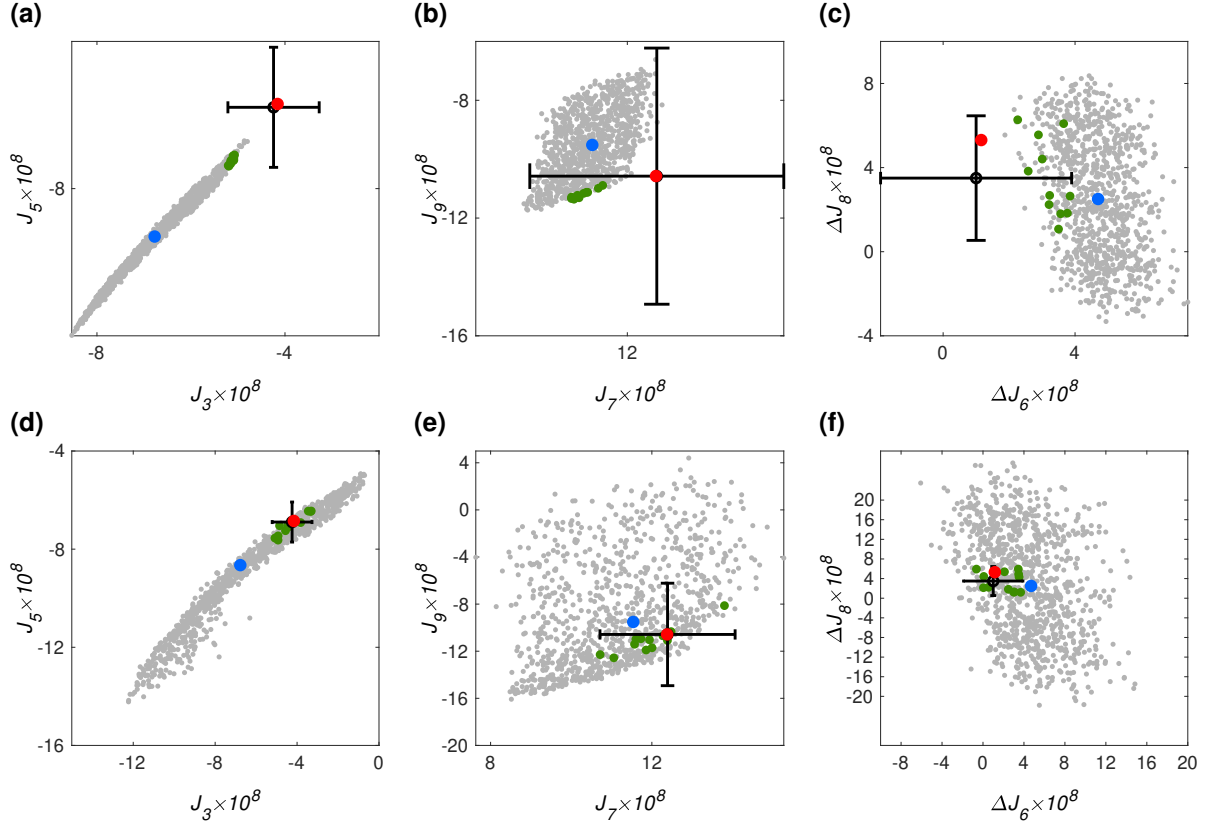

Figure S7: Solutions with random winds, similar to Fig. 4 in main text, but with different strength of the random winds. (a-c) Solutions with random winds that are half as strong. (d-f) Solutions with random winds that are twice as strong. Shown are the solutions with 1000 random cases (gray), and those of which the solution matches all the gravity harmonics (green). The plausible solutions (green) constitute 1% of the total cases in the upper panels, and 1.2% in the lower panels. Also shown are the solution with no random winds (blue, corresponding to the  $25^\circ$  case in Fig. 3 in the main text), the solution with no truncation of the winds (red, corresponding to the  $90^\circ$  case in Fig. 3 in the main text) and the measurements (black).

## References

- Cao, H., and D. J. Stevenson, Zonal flow magnetic field interaction in the semi-conducting region of giant planets, *Icarus*, *296*, 59–72, doi:10.1016/j.icarus.2017.05.015, 2017.
- Galanti, E., and Y. Kaspi, An Adjoint-based Method for the Inversion of the Juno and Cassini Gravity Measurements into Wind Fields, *Astrophys. J.*, *820*(2), 91, doi:10.3847/0004-637X/820/2/91, 2016.
- Galanti, E., and Y. Kaspi, Combined magnetic and gravity measurements probe the deep zonal flows of the gas giants, *MNRAS*, *501*(2), 2352–2362, doi:10.1093/mnras/staa3722, 2021.
- Galanti, E., Y. Kaspi, and E. Tziperman, A full, self-consistent treatment of thermal wind balance on oblate fluid planets, *J. Fluid Mech.*, *810*, 175–195, doi:10.1017/jfm.2016.687, 2017.
- Iess, L., et al., Measurement of Jupiter’s asymmetric gravity field, *Nature*, *555*, 220–222, doi:10.1038/nature25776, 2018.
- Kaspi, Y., Inferring the depth of the zonal jets on Jupiter and Saturn from odd gravity harmonics, *Geophys. Res. Lett.*, *40*, 676–680, doi:10.1029/2009GL041385, 2013.
- Kaspi, Y., G. R. Flierl, and A. P. Showman, The deep wind structure of the giant planets: Results from an anelastic general circulation model, *Icarus*, *202*(2), 525–542, doi:10.1016/j.icarus.2009.03.026, 2009.
- Kaspi, Y., J. E. Davighi, E. Galanti, and W. B. Hubbard, The gravitational signature of internal flows in giant planets: comparing the thermal wind approach with barotropic potential-surface methods, *Icarus*, *276*, 170–181, 2016.
- Kaspi, Y., E. Galanti, A. P. Showman, D. J. Stevenson, T. Guillot, L. Iess, and S. J. Bolton, Comparison of the Deep Atmospheric Dynamics of Jupiter and Saturn in Light of the Juno and Cassini Gravity Measurements, *Space Sci. Rev.*, *216*(5), 84, doi:10.1007/s11214-020-00705-7, 2020.
- Kaspi, Y., et al., Jupiter’s atmospheric jet streams extend thousands of kilometres deep, *Nature*, *555*, 223–226, doi:10.1038/nature25793, 2018.
- Liu, J., T. Schneider, and Y. Kaspi, Predictions of thermal and gravitational signals of Jupiter’s deep zonal winds, *Icarus*, *224*, 114–125, 2013.
- Pedlosky, J., *Geophysical Fluid Dynamics*, pp. 710. Springer-Verlag, 1987.
- Tollefson, J., et al., Changes in Jupiter’s zonal wind profile preceding and during the Juno mission, *Icarus*, *296*, 163–178, doi:10.1016/j.icarus.2017.06.007, 2017.
- Zhang, K., D. Kong, and G. Schubert, Thermal-gravitational Wind Equation for the Wind-induced Gravitational Signature of Giant Gaseous Planets: Mathematical Derivation, Numerical Method, and Illustrative Solutions, *Astrophys. J.*, *806*(2), 270, doi:10.1088/0004-637X/806/2/270, 2015.
